# Supplementary material for: Learning the Electrostatic Response of the Electron Density through a Symmetry-Adapted Vector Field Model
Source: arXiv:2501.11019 ancillary file (2025-02-25)
Supplement: Supplementary file 1 [file SI.pdf]

# Learning the Electrostatic Response of the Electron Density through a Symmetry-Adapted Vector Field Model - Supporting Information

Mariana Rossi,[1] Kevin Rossi,[2,3] Alan M. Lewis,[4] Mathieu Salanne,[5,6] and Andrea Grisafi[6,*]

[1] *Max Planck Institute for the Structure and Dynamics of Matter, Luruper Chaussee 149, 22761 Hamburg, Germany*
[2] *Department of Materials Science and Engineering, Delft University of Technology, 2628 CD, Delft, The Netherlands*
[3] *Climate Safety and Security Centre, TU Delft The Hague Campus, Delft University of Technology, 2594 AC, The Hague, The Netherlands*
[4] *Department of Chemistry, University of York, Heslington, York, YO10 5DD, UK*
[5] *Institut Universitaire de France (IUF), F-75231 Paris, France*
[6] *Physicochimie des Électrolytes et Nanosystèmes Interfaciaux, Sorbonne Université, CNRS, F-75005 Paris, France*

[*] andrea.grisafi@sorbonne-universite.fr

## I. DERIVATION OF SYMMETRY-ADAPTED $\lambda \otimes 1$ KERNELS

Consider the expansion of a vectorial field on an atom-centered basis $\phi$ made of radial functions and orthonormalized real spherical harmonics. Assuming for simplicity a non-periodic system, we have

$$\frac{\partial n_e(\boldsymbol{r})}{\partial E_k} = \sum_{in\lambda\mu} c^k_{in\lambda\mu} \phi_{in\lambda\mu}(\boldsymbol{r} - \boldsymbol{r}_i) \tag{S1}$$

where $k$ are the Cartesian indexes $x, y, z$. We would like to approximate the expansion coefficients using an equivariant kernel-based ansatz. For that, we can rely on the fact that a Cartesian vector follows the same transformation rules of a real spherical harmonics of order 1. To derive the symmetry-adapted kernel, it is convenient to work in complex space, so that to rely on known rules of composition of angular momenta, and apply the complex to real unitary transformation matrices for spherical harmonics of order $\lambda$ and 1 at the final step in derivation. From this prescription, we can define the complex kernel function that expresses the rotational symmetry of the vectorial field components from the following rotational average:

$$K^{\lambda\otimes 1}_{\mu k,\mu' k'}(i,j) = \int_{SO(3)} d\hat{R}\; D^{\lambda}_{\mu\mu'}(\hat{R}) D^{1}_{kk'}(\hat{R}) \left| \int d\boldsymbol{r} \chi_i(\boldsymbol{r}) \chi'_j(\mathbf{R}\boldsymbol{r}) \right|^2 \tag{S2}$$

where we left the freedom of adopting two different types of atomic environments representations $\chi$ and $\chi'$. Following Ref. 1, one can then expand $\chi$ and $\chi'$ in spherical harmonics centered about the atoms $i$ and $j$. Upon doing the math, one is ultimately left with having to perform the following integral over four Wigner $D$-matrices:

$$\int_{SO(3)} d\hat{R}\; D^{\lambda}_{\mu\mu'}(\hat{R}) D^{1}_{kk'}(\hat{R}) D^{l,\star}_{mm'}(\hat{R}) D^{l'}_{m''m'''}(\hat{R}) \tag{S3}$$

While this looks complex, we can rely on the following irreducible decomposition:

$$D^{\lambda}_{\mu\mu'} D^{1}_{kk'} = \sum_{L=|\lambda-1|}^{\lambda+1} \langle \lambda\mu, 1k | L, \mu+k \rangle \langle \lambda\mu', 1k' | L, \mu'+k' \rangle\, D^{L}_{(\mu+k)(\mu'+k')} \tag{S4}$$

Notably, by bringing the sum over irreducible components outside, one falls back into the standard derivation of spherical kernels covariant in $SO(3)$, obtaining

$$K^{\lambda\otimes 1}_{\mu k,\mu' k'}(i,j) = \sum_{L=|\lambda-1|}^{\lambda+1} \langle \lambda\mu, 1k | L, \mu+k \rangle \langle \lambda\mu', 1k' | L, \mu'+k' \rangle\, K^{L}_{(\mu+k)(\mu'+k')}(i,j) \tag{S5}$$

From this result, symmetrization under inversion operations $\hat{\boldsymbol{\imath}}$ implies

$$K^{\lambda\otimes 1, O(3)}_{\mu k,\mu' k'}(i,j) = K^{\lambda\otimes 1}_{\mu k,\mu' k'}(i,j) + (-1)^{\lambda+1} K^{\lambda\otimes 1}_{\mu k,\mu' k'}(i,\hat{\boldsymbol{\imath}}\, j) \tag{S6}$$

and therefore, for each $L$,

$$\tilde{K}^{L}_{(\mu+k)(\mu'+k')}(i,j) = K^{L}_{(\mu+k)(\mu'+k')}(i,j) + (-1)^{\lambda+1} K^{L}_{(\mu+k)(\mu'+k')}(i,\hat{\boldsymbol{\imath}}\, j) \tag{S7}$$

From the definition of $\boldsymbol{K}^L$, this implies the following symmetrization rule of the rotationally covariant structural descriptor of order $L$:

$$\begin{aligned} \tilde{\boldsymbol{P}}^{L}_{aa'nn'll'}(i) &= \boldsymbol{P}^{L}_{aa'nn'll'}(i) + (-1)^{\lambda+1} \boldsymbol{P}^{L}_{aa'nn'll'}(\hat{\boldsymbol{\imath}}\, i) \\ &= \boldsymbol{P}^{L}_{aa'nn'll'}(i) + (-1)^{\lambda+1+l+l'} \boldsymbol{P}^{L}_{aa'nn'll'}(i) \\ &= \boldsymbol{P}^{L}_{aa'nn'll'}(i) \left[1 + (-1)^{\lambda+1+l+l'}\right] \end{aligned} \tag{S8}$$

where $\boldsymbol{P}^{L}_{aa'nn'll'}$ is a vector of size $3 \times (2\lambda+1)$. From the previous result, only those structural features for which $l + l' + \lambda + 1$ is even survive. In practice, this implies that, for $L = |\lambda \pm 1|$ we must consider combination of indexes for which $l + l' + L$ is even, exactly as in the standard $O(3)$ kernels, while for $L = \lambda$ we must consider the combination of indexes for which $l + l' + L$ is odd. We note that, when considering the special case of $\lambda = 0$, the Clebsch-Gordan coefficients give $\delta_{1L}\delta_{kM}$, so that we are left with the conventional $L = 1$ spherical tensor kernels.

## II. VECTOR-FIELD LEARNING MODEL

By directly extending what done within the SALTED method for electron density predictions [2], the kernels previously derived can be used to perform equivariant predictions of the density-response expansion coefficients via the following linear combination:

$$c^{k}_{in\lambda\mu} = \sum_{j=1}^{M(\lambda)} \sum_{\mu' k'} w^{k'}_{jn\lambda\mu'} \, K^{\lambda\otimes 1}_{\mu k,\mu' k'}(i,j) \, \delta_{a_i a_j} \tag{S9}$$

where $w^{k'}_{jn\lambda\mu'}$ are the regression weights, defined to depend on the Cartesian coordinate $k$. The index $j$ runs over a sparse set of $M_\lambda$ atomic environments of chemical species $a_j$, defined in this work to decrease with increasing angular momenta according to a Gaussian decay factor, i.e., $M_\lambda = M_0 e^{-0.05\lambda}$, with $M_0$ an input parameter. The same procedure used for the electron density is then used to recast the problem into a truncated reproducing kernel Hilbert space (RKHS), allowing us to numerically stabilize the learning procedure [2].

Upon this procedure, the RKHS regression weights $\boldsymbol{w}$ can be found by minimizing a loss function that measures the integrated mean square error between the reference and predicted electrostatic responses. As a key difference with respect to the case of electron densities, this is done by collecting contribution not only from $N$ training configurations, but also from each of the three Cartesian components of the electron-density response. In fact, this aspect is crucial to guarantee equivariance of the learning procedure under an arbitrary three-dimensional rotation of the training structures. In compact notation, we can then write the vector-field loss function as follows:

$$\mathcal{L}(\boldsymbol{w}) = \sum_{I=1}^{N} \left[ \sum_{k} \Delta \boldsymbol{c}^{k}_{I}(\boldsymbol{w}) \cdot \mathbf{S}_I \cdot \Delta \boldsymbol{c}^{k}_{I}(\boldsymbol{w}) \right] + \eta \, \|\boldsymbol{w}\|^2 \, , \tag{S10}$$

where $\Delta \boldsymbol{c}^{k}_{I}$ are the difference vectors between quantum-mechanical and predicted coefficients for a given structure $I$ and Cartesian component $k$, $\mathbf{S}_I$ is the overlap matrix between basis functions for the corresponding structure, defined to be independent from $k$, and $\eta$ is a regularization parameter.

## III. DATASET GENERATION

We report here information about the reference DFPT and finite-field DFT calculations performed to compute the datasets of density-response expansion coefficients used to train and test the vector-field learning model.

### A. Water monomer

The geometries of the water monomer dataset were obtained from Refs. 1, 3. The density-response data and corresponding RI expansion coefficients [4] were generated with the PBE functional and *light* defaults for the atom-centered basis-sets and numerical grids with the FHI-aims code [5]. The `DFPT dielectric` keyword was used to obtain the density response, because the dataset contains water molecules in a box with periodic boundary conditions. An input-file example for this data generation can be found in the SALTED repository.

### B. Liquid water and naphtalene crystals

We refer to Ref. 3 for details about the dataset generation, which used the electric-field DFPT implementation in the FHI-aims code, with similar settings to the water monomer dataset.

### C. Gold nanoparticles

All of the 255 gold nanoparticles geometries – plus the additional 30 used to test the method under extrapolation conditions – were relaxed (in isolation) with the PBE functional using the FHI-aims code package, adopting *light* setting for basis sets and numerical grids. In order to be able to profit from the analytical expressions to calculate integrals involving the predicted density coefficients when working with Gaussian basis sets, we switch to the CP2K

program [6] to compute the training data. We obtain reference calculations of the density response by finite differences under applied electric fields of 0.01V/Å along the three Cartesian directions. Specifically, we run finite-field calculations at the DFT/PBE level [7] with a ccGRB-T basis and GTH pseudopotentials [8]. A Martyna-Tuckerman correction is also applied to screen the dipolar interaction between the periodic images of the system. [9] Finally, we adopt the resolution of the identity (RI) method based on an overlap metric, as implemented in CP2K [10], to represent the electron density and compute the response coefficients by finite differences.

## IV. MACHINE-LEARNING PARAMETERS

We report here the machine-learning parameters used to produce the result of this work. In all cases, rotationally invariant $\lambda = 0$ kernels are multiplied by the $\lambda \otimes 1$ (vector-field) kernels in order to increase the degree of nonlinearity of the learning model, following a $\zeta = 2$ kernel exponentiation.

### A. Water monomers

Symmetry-adapted $\lambda \otimes 1$ kernels were constructed starting from 3-body $\lambda$-SOAP features [1], i.e., $|\rho \otimes \rho \otimes \lambda\mu\rangle$. For that, the atom-density $\rho$ is defined using a Gaussian width of $\sigma = 0.3$ Å within a radial cutoff of $r_{\text{cut}} = 4.0$ Å, projected onto 8 Gaussian-type radial functions and spherical harmonics up to $l = 6$. $M_0 = 100$ sparse atomic environments were selected to reduce the RKHS size. A value of $\eta = 10^{-8}$ was chosen as a regularization parameter.

### B. Liquid water and naphthalene crystals

The $\lambda$-SOAP atom-density representations of both liquid water and naphthalene were calculated using a Gaussian width of $\sigma = 0.3$ Å and a radial cutoff of $r_{\text{cut}} = 4.0$ Å, and projected onto 8 Gaussian-type functions and spherical harmonics up to $l = 6$. For the SALTER calculations a regularization parameter of $\eta = 10^{-8}$ was used, while for the equivariant models it was set to $\eta = 10^{-6}$. For the SALTER model of bulk water $M = 3000$ reference environments were selected to reduce the RKHS, whereas for the SALTER model of naphthalene $M = 2000$ reference environments were chosen. In SALTER calculations, the same number of environments are used for each value of $\lambda$, unlike the equivariant models where fewer environments are chosen as $\lambda$ increases. For the equivariant models of both bulk water and naphthalene, $M_0 = 500$ was used.

### C. Gold nanoparticles

Symmetry-adapted $\lambda \otimes 1$ kernels were constructed starting from a multiscale long-distance equivariant (LODE) representation of the atomic environment as described in Ref. 11, i.e., $|\rho \otimes V \otimes \lambda\mu\rangle$. Specifically, the atom-density $\rho$ is defined using a Gaussian width of $\sigma = 0.5$ Å within a radial cutoff of $r_{\text{cut}} = 10.0$ Å, projected onto 8 Gaussian-type functions and spherical harmonics up to $l = 6$, while the atomic potential $V$ is defined using a Gaussian width of $\sigma = 2.0$ Å within a radial cutoff of $r_{\text{cut}} = 10.0$ Å, projected onto 4 Gaussian-type functions and spherical harmonics up to $l = 3$. $M_0 = 200$ sparse atomic environments were selected to reduce the RKHS size. A value of $\eta = 10^{-5}$ was chosen as a regularization parameter.

## V. CALCULATION OF POLARIZABILITY TENSOR

For nonperiodic systems, the polarizability tensor can be analytically computed from the predicted density-response function. Starting from the linear atom-centered representation of the electron density response, in particular, we obtain that only $\lambda = 0$ and $\lambda = 1$ spherical harmonics coefficients contribute to the calculation of $\boldsymbol{\alpha}$. Assuming real spherical harmonics, the derivation reads as follows:

$$
\begin{aligned}
\alpha_{kk'} &= \int_{\mathcal{R}^3} d\boldsymbol{r}\, \boldsymbol{r}_k \frac{\partial n_e(\boldsymbol{r})}{\partial E_{k'}} \\
&= \int_{\mathcal{R}^3} d\boldsymbol{r}\, \boldsymbol{r}_k \left[ \sum_i \sum_{n\lambda\mu} c^{k'}_{in\lambda\mu} R^{\lambda}_n(|\boldsymbol{r}-\boldsymbol{r}_i|) Y_{\lambda\mu}(\widehat{\boldsymbol{r}-\boldsymbol{r}_i}) \right] \\
&= \sum_i \sum_{n\lambda\mu} c^{k'}_{in\lambda\mu} \int_{\mathcal{R}^3} d\boldsymbol{r}\, (\boldsymbol{r}-\boldsymbol{r}_i+\boldsymbol{r}_i)_k\, R^{\lambda}_n(|\boldsymbol{r}-\boldsymbol{r}_i|) Y_{\lambda\mu}(\widehat{\boldsymbol{r}-\boldsymbol{r}_i}) \\
&= \sum_i \sum_{n\lambda\mu} c^{k'}_{in\lambda\mu} \left[ r^k_i \sqrt{4\pi}\delta_{\lambda 0}\delta_{\mu 0} \int_0^\infty dr\, r^2 R^{\lambda}_n(r) + \sqrt{\frac{4\pi}{3}} \delta_{\lambda 1}\delta_{\mu k} \int_0^\infty dr\, r^3 R^{\lambda}_n(r) \right] \\
&= \sum_i \sum_n \left[ r^k_i\, c^{k'}_{in00} \sqrt{4\pi} \int_0^\infty dr\, r^2 R^0_n(r) + c^{k'}_{in1k} \sqrt{\frac{4\pi}{3}} \int_0^\infty dr\, r^3 R^1_n(r) \right] ,
\end{aligned}
\tag{S11}
$$

where we adopted the correspondence between Cartesian versors and $\lambda = 1$ real spherical harmonic components $k$, i.e., $(\hat{x}, \hat{y}, \hat{z}) \to (1, -1, 0)$. We note that the equality reported in the first line of Eq. (S11) is derived from the Helmann-Feynman theorem under the hypothesis of a normalized charge-density distribution. From a practical point of view, this implies that, for each Cartesian components $k'$, the predicted $\lambda = 0$ coefficients must be rescaled to ensure that the density response function integrates exactly to zero. This procedure is equivalent to what implemented in Ref. 2 to guarantee a physically consistent calculation of the induced polarization vector based on predicted electron density variations. In fact, by dropping the $k'$ index everywhere, the formula so derived can directly be applied for computing the electronic contribution to the dipole moment in nonperiodic systems. Finally, we note that thanks to the choice of Gaussian-type basis functions used within the RI approximation of CP2K, we are able to exploit analytical formulas to compute the radial integrals entering the last line of Eq. (S11). However, numerical atomic orbitals could in principle also be adopted by evaluating those integrals on suitable 1D meshes.

## VI. COMPLEMENTARY RESULTS FOR AU NANOPARTICLES

We report in Figure S1 the predicted isotropic component ($\alpha_0$) of the polarizability of the gold nanoparticles as a function of the number of gold atoms. We note how a vector field model that relies on a nonlocal description of the atomic environment is essential to accurately reproduce the linear increase of $\alpha_0$ for the largest nanoparticles used to validate the model under extrpolation conditions.

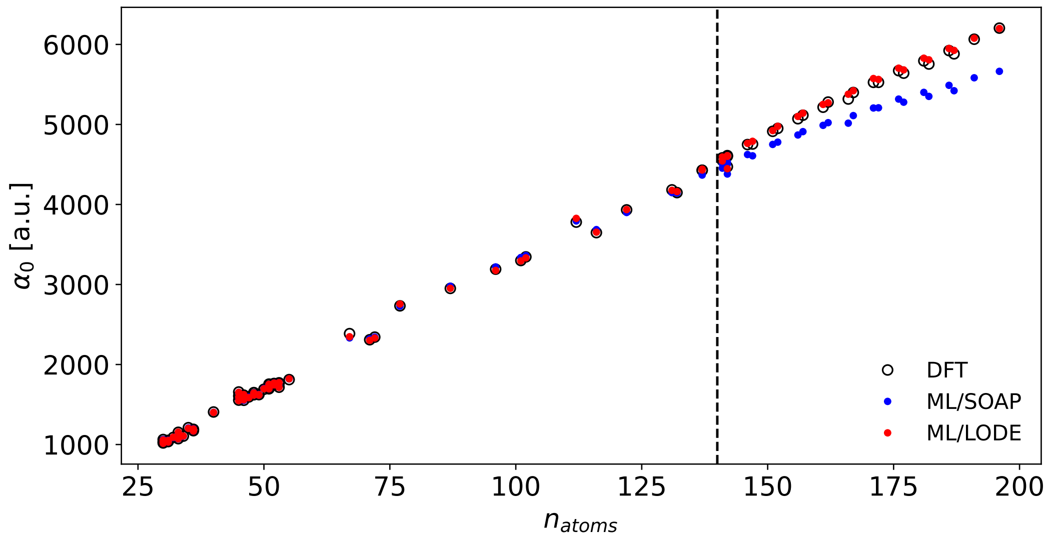


Figure S1: Isotropic components ($\alpha_0$) of the polarizability tensors of 85 gold nanoparticles of increasing size, as obtained from the corresponding electron density response coefficients. Empty circles: DFT reference. Red dots: ML/LODE prediction. Blue dots: ML/SOAP prediction. The dashed line separates the domain of sizes used for training the vector-field model ($n_{\mathrm{atoms}} < 140$) from the large-scale domain of sizes used to validate the model under extrapolation conditions ($n_{\mathrm{atoms}} > 140$).

We report in Figure S2 the predicted anisotropic component ($\alpha_{\mathrm{aniso}}$) of the polarizability of the gold nanoparticles dataset against the refence DFT values, defined as the Forbenius norm of the traceless $\boldsymbol{\alpha}$-tensor. Paradigmatic examples are reported as insets of the Figure: while an octahedral configuration display an isotropic polarizability, a Marks decahedron structure [12] shows a substantial cross response between the $z$-axis and the $xy$-plane. Our method displays a high level of correlation across the entire regime of sizes, including the extrapolation domain ($n_{\mathrm{atoms}} > 140$), which is associated with a 11.9% RMSE measured with respect to the standard deviation of $\alpha_{\mathrm{aniso}}$ in the test set.

For completeness, we also report in Figures S3 the absolute errors associated with the indirect prediction of both isotropic and anisotropic polarizability components as a function of the number of Au atoms.

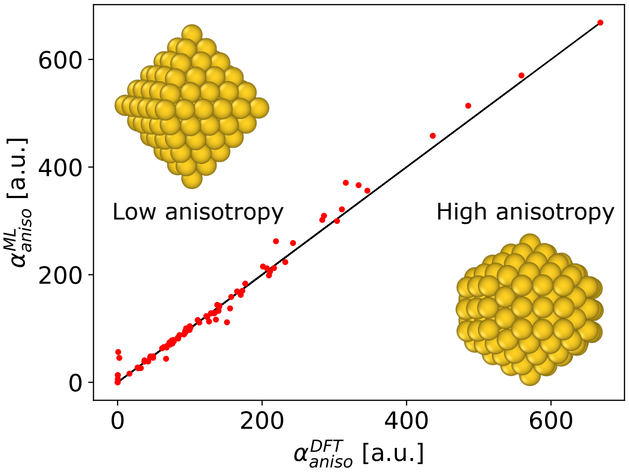


Figure S2: Correlation plot between reference (DFT) and predicted (ML) anisotropic part of the polarizability tensor, $\alpha_{\text{aniso}}$, as indirectly computed from reference and predicted electron-density response coefficients, respectively. An octahedral geometry and a Marks decahedral geometry are reported as examples of a low and high level of anisotropy, respectively.

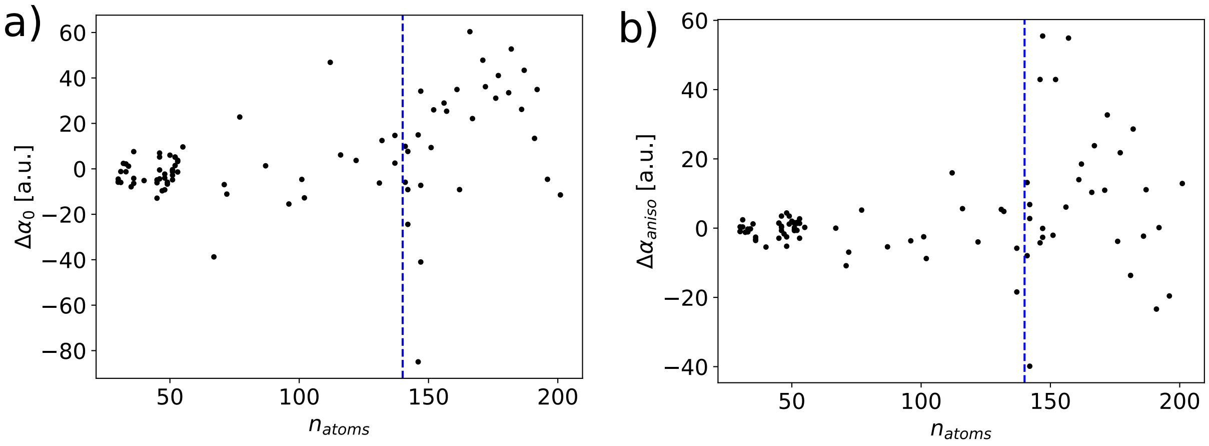


Figure S3: Absolute errors of isotropic (a) and anisotropic (b) components of the polarizability tensor, as computed from the deviation between reference and predicted density-response coefficients. The dashed blue line separates the training domain of nanoparticle sizes ($n_{\text{atoms}} < 140$) from the extrapolation domain ($n_{\text{atoms}} > 140$).

[S1] Andrea Grisafi, David M. Wilkins, Gábor Csányi, and Michele Ceriotti. Symmetry-Adapted Machine Learning for Tensorial Properties of Atomistic Systems. *Phys. Rev. Lett.*, 120(3):036002, January 2018.

[S2] Andrea Grisafi, Alan M. Lewis, Mariana Rossi, and Michele Ceriotti. Electronic-structure properties from atom-centered predictions of the electron density. *Journal of Chemical Theory and Computation*, 19(14):4451–4460, 2023.

[S3] Alan M. Lewis, Paolo Lazzaroni, and Mariana Rossi. Predicting the electronic density response of condensed-phase systems to electric field perturbations. *The Journal of Chemical Physics*, 159(1):014103, 07 2023.

[S4] Xinguo Ren, Patrick Rinke, Volker Blum, Jürgen Wieferink, Alexandre Tkatchenko, Andrea Sanfilippo, Karsten Reuter, and Matthias Scheffler. Resolution-of-identity approach to Hartree-Fock, hybrid density functionals, RPA, MP2 and GW with numeric atom-centered orbital basis functions. *New J. Phys.*, 14:053020, 2012.

[S5] Volker Blum, Ralf Gehrke, Felix Hanke, Paula Havu, Ville Havu, Xinguo Ren, Karsten Reuter, and Matthias Scheffler. Ab initio molecular simulations with numeric atom-centered orbitals. *Comput. Phys. Commun.*, 180(11):2175–2196, 2009.

[S6] Thomas D. Kühne, Marcella Iannuzzi, Mauro Del Ben, Vladimir V. Rybkin, Patrick Seewald, Frederick Stein, Teodoro Laino, Rustam Z. Khaliullin, Ole Schütt, Florian Schiffmann, Dorothea Golze, Jan Wilhelm, Sergey Chulkov, Mohammad Hossein Bani-Hashemian, Valéry Weber, Urban Borštnik, Mathieu Taillefumier, Alice Shoshana Jakobovits, Alfio

Lazzaro, Hans Pabst, Tiziano Müller, Robert Schade, Manuel Guidon, Samuel Andermatt, Nico Holmberg, Gregory K. Schenter, Anna Hehn, Augustin Bussy, Fabian Belleflamme, Gloria Tabacchi, Andreas Glöß, Michael Lass, Iain Bethune, Christopher J. Mundy, Christian Plessl, Matt Watkins, Joost VandeVondele, Matthias Krack, and Jürg Hutter. Cp2k: An electronic structure and molecular dynamics software package - quickstep: Efficient and accurate electronic structure calculations. *The Journal of Chemical Physics*, 152(19):194103, 2020.

[S7] Jp P Perdew, K Burke, and M Ernzerhof. Generalized Gradient Approximation made simple. *Phys. Rev. Lett.*, 77(18):3865, 1996.

[S8] S. Goedecker, M. Teter, and J. Hutter. Separable dual-space gaussian pseudopotentials. *Phys. Rev. B*, 54:1703–1710, Jul 1996.

[S9] Glenn J. Martyna and Mark E. Tuckerman. A reciprocal space based method for treating long range interactions in ab initio and force-field-based calculations in clusters. *The Journal of Chemical Physics*, 110(6):2810–2821, 1999.

[S10] Augustin Bussy, Ole Schütt, and Jürg Hutter. Sparse tensor based nuclear gradients for periodic Hartree–Fock and low-scaling correlated wave function methods in the CP2K software package: A massively parallel and GPU accelerated implementation. *The Journal of Chemical Physics*, 158(16):164109, 2023.

[S11] Andrea Grisafi, Jigyasa Nigam, and Michele Ceriotti. Multi-scale approach for the prediction of atomic scale properties. *Chem. Sci.*, 12:2078–2090, 2021.

[S12] L.D. Marks. Modified wulff constructions for twinned particles. *Journal of Crystal Growth*, 61(3):556–566, 1983.
